# Supplementary material for: Almost Free: Self-concordance in Natural Exponential Families and an Application to Bandits
Source: arXiv:2410.01112 source file (2024-10-01)
Supplement: Supplementary file 1 [file notations.tex]

\section{Notations, symbols and definitions}
\subsection{Notations}
Let $\cV$ be a subset of the reals. For a function $f:\cV\to\RR$ that is three-times differentiable on $\cV^\circ$, the interior of $\cV$, we use $\dot f$, $\ddot f$ and $\dddot f$ to denote their first, second and third order derivatives. For $n\in \NN^+$, we denote $[n]:=\{1,2,\dotsc, n\}$. For $d\in \NN^+$, a vector $x\in \RR^d$ and a positive definite matrix $M\in \RR^{d\times d}$, we denote the $\ell_2$-norm weighted by $M$ as $\|x\|_{M}=\sqrt{x^\top Mx}$. We denote $\|\cdot\|$ as the $\ell_2$-norm and for the normed space $(\RR^d, \|\cdot\|)$, the $d$-dimensional closed unit ball is denoted as $B_2^d:=\{x\in \RR^d:\|x\|\le 1\}$.
\subsection{Symbols and definitions}\label{section:appendix_symbols}
We keep a collection of symbols and definitions that will be used across the whole appendix.
\paragraph{Natural Exponential Family}
For a distribution $P$ on $\RR$, we denote the moment generating function of $P$ as
\begin{equation*}
    M_P(u)=\int_\RR \exp(uy)P(dy)
\end{equation*}
and the cumulant generating function as $\psi_P(u)=\log M_P(u)$.
For a distribution $Q$ on the reals, the (exponentially) tilted distribution $Q_u$ is defined to be 
\begin{equation*}
    Q_u(dy)=\frac{1}{M_Q(u)}\exp(uy)Q(dy),
\end{equation*}
and $u$ is referred to as the tilting parameter.
A natural exponential family $\cQ$ with base distribution $Q$ takes the following term:
\begin{equation*}
    \cQ = \{Q_u(dy):u\in \cU_Q\},
\end{equation*}
where $\cU_Q=\{u\in \RR: \psi_Q(u)<\infty\}$.
The cumulant generating function of $Q$, $\psi_Q(u)$, is also referred to as the cumulant function of $\cQ$. We use $\mu(u)=\int_\RR yQ_u(dy)$ to denote the mean of $Q_u$ for $u\in \cU_Q$. 
Given a set $\cU\subseteq \cU_Q$ where $0\in \cU^\circ$, we can also consider another natural exponential family on $\cU$:
\begin{equation*}
    (Q_u)_{u\in \cU}:=\{Q_u(dy):u\in \cU\}\subseteq \cQ.
\end{equation*}
To show that certain NEFs possess the self-concordance property, we will be analyzing the following quantity:
\begin{equation*}
    \selfconc_Q(u)=\frac{\int |y-\mu(u)|^3Q_u(dy)}{\int (y-\mu(u))^2Q_u(dy)}.
\end{equation*}
\cref{prop:moments_of_NEF} captures useful properties of NEFs.
\paragraph{Generalized Linear Bandits}
We consider bandits where the reward of each arm comes from the same NEF with different tilting parameters. To be more specific, as is described in \cref{ass:se}, the base distribution $Q$ has subexponential tails:
there exists $c_1,C_1,C_2\in (0,\infty)$ and $c_2\in (0,\infty]$ such that for all $y\in \RR^+$,
\begin{align*}
    Q([y,\infty))\le C_1\exp(-c_1y), Q((-\infty,y])\le C_2\exp(-c_2y).
\end{align*}
The reward of each arm $x\in \cX$ is from $Q_{x^\top\theta_\star}$ where $\theta_\star\in \Theta$ is an unknown true underlying distribution.
Recall given a list of pairs $\cD=(X_i,Y_i)_{i=1}^s\subset \RR^d\times \RR$, the negative $\lambda$-regularized log-likelihood for $\lambda \ge 0$ is defined to be
\begin{align*}
    \cL(\theta;\cD,\lambda)&=\frac{\lambda}{2}\|\theta\|^2-\sum_{i=1}^s \log q(Y_i;X_i^\top\theta)\\
    &=\frac{\lambda}{2}\|\theta\|^2-\sum_{i=1}^s(Y_iX_i^\top\theta-\psi_Q(X_i^\top\theta)),
\end{align*}
where for $u\in \cU$, $q(;u)=\frac{dQ_u}{dQ}$ is the Radon-Nikodym derivative.
We will need the Hessian of the negative $\lambda$-regularized log-likelihood 
\begin{equation*}
    H_t(\theta)=\nabla^2 \cL(\theta;\cD,\lambda)=\sum_{i=1}^t \dot\mu(X_i^\top\theta)X_iX_i^\top+\lambda I.
\end{equation*}
% We introduce the difference quotient of $\mu(\cdot)$ to help reason about $H_t(\theta)$. For $u\neq u'\in \cU_Q^\circ$, define
% \begin{equation*}
%     \alpha(u,u')=\frac{\mu(u)-\mu(u')}{u-u'}.
% \end{equation*}
Note that by definition of derivative, we have that $\lim_{u'\to u}\alpha(u,u')=\dot\mu(u)$.
% , hence $\alpha(\cdot,\cdot)$ is also a secant approximation to $\dot\mu(\cdot)$. 
The difference quotient $\alpha(\cdot, \cdot)$ can also be viewed as the $0$-th order remainder of the Taylor expansion of $\mu(\cdot)$, whose integral form is $\alpha(u,u')=\int_0^1\dot\mu(u+v(u'-u))dv$.
Clearly $\alpha$ is symmetric w.r.t. its own arguments, i.e., $\alpha(u,u')=\alpha(u',u)$ for $u\neq u'\in \cU_Q^\circ$.
Based on the difference quotient, for $\theta_1, \theta_2\in \Theta$, we define
\begin{equation*}
    G_t(\theta_1,\theta_2)=\lambda I + \sum_{i=1}^t \alpha(X_i^\top\theta_1,X_i^\top\theta_2)X_iX_i^\top .
\end{equation*}
To approximate $H_t(\theta)$, for $\theta_1,\theta_2\in \RR^d$, we also introduce
\begin{equation*}
    G_t(\theta_1,\theta_2)=\sum_{i=1}^t \alpha(X_i^\top\theta_1, X_i^\top\theta_2)X_iX_i^\top+\lambda I
\end{equation*} 

For all $\theta$ in the admissible parameter set $\Theta$, there exists $S_1>0$, $S_3>-c_2$ and $S_2<c_1$ such that for all $x\in \cX$ it follows that 
\begin{equation*}
    \|\theta\|\le S_1, S_3\le x^\top\theta\le S_2
\end{equation*}
We define $g_t:\Theta\to\RR^d$ that will be used in analysis as well as confidence set construction to be 
\begin{equation*}
    g_t(\theta)=\sum_{i=1}^t \mu(X_i^\top\theta)X_i+\lambda \theta.
\end{equation*}
